# Supplementary material for: String Diagram Rewrite Theory III: Confluence with and without Frobenius
Source: arXiv:2109.06049 source file (2022-04-18)
Supplement: Supplementary file 1 [file appendixConvexity.tex]

The whole proof goes through like for Theorem \ref{th:locconfl} apart from one crucial step: when extracting the critical pair (Construction~\ref{constr:extraction}), we cannot let the interface $J'$ be given by pullback (Example~\ref{ex:badpullback}). This is also problematic for the application of Lemma~\ref{lemmacube}, which relies on the fact that $J'$ is constructed as a pullback. Fortunately, mda-hypergraphs are extremely well-behaved and the following property can be used to solve these issues.

\begin{lem}\label{lemma:keyconvex}
 Let $(G'\tl{f'}J')$ and $(G\tl{f}J)$ be two mda-hypergraphs with interfaces. Suppose that $f'$ is mono. If there exists a mono $m\colon G' \to G$ then there exist a $\Sigma$-hypergraph $C$ and morphisms $J'\tr{}C$ and $J\tr{}C\tr{}G$ making the following diagram commute and the square $(\dagger)$ below a pushout.
\begin{equation*}\label{diag:embeddingAssumptionnew}
\begin{aligned}
\xymatrix{
& J' \ar[r]^{f'} \ar[d] \ar@{}[dr]|(.5){(\dagger)} & G' \ar[d]^m \\
J  \ar[r]  \ar@/_10pt/[rr]_f 
& C  \ar[r] & G
}
\end{aligned}
\end{equation*}
\end{lem}
\begin{proof}
For a hypergraph $H$, we let $V_H$ and $E_H$ denote its sets of nodes and hyperedges. %, respectively. 

We define $C$ as the $\Sigma$-hypergraph having as set of nodes $V_G \setminus m(V_{G'} \setminus f'(V_{J'}))$ and as set of hyperedges $E_G \setminus m(E_{G'})$. Then, there are evident embeddings of $J'$ into $C$ and $C$ into $G$. For $m$ and $f'$ mono, this is the standard calculation of the pushout complement, so to prove that $(\dagger)$ is a pushout we need only show that $C$ is well-defined. This is true whenever $m$ satisfies the gluing conditions, namely no hyperedge in $E_G \setminus  m(E_{G'})$ has a source or target in $V_G \setminus m(V_{G'} \setminus f'(V_{J'}))$. Now, nodes $v$ in $V_{G'} \setminus f'(V_{J'})$ are internal nodes of $G'$, so by monogamy, $m(v)$ must have a unique in- and out-hyperedge, both in the image of $m$. In particular, these hyperedges cannot be in $E_G \setminus  m(E_{G'})$.

To prove the statement we only need to show the existence of $J\tr{g}C$ making the lower part of the above diagram commute. 
We can take $g(v)= f(v)$ for all vertex $v \in J$. This is well defined since $f(v) \notin m(V_{G'} \setminus f' (V_{J'}))$: as discussed above, all nodes $v' \in V_{G'} \setminus f'(V_{J'})$ should be internal in $G$, so by monogamy $m(v')$ should have exactly one in and out hyperedge and it cannot be in the image of the interface $J$.
\end{proof}

\begin{proof}[Proof of Theorem~\ref{th:locconflwellformed}]
 By assumption we have two rewriting steps from $(G_0\tl{} I)$.
$$\xymatrix@R=15pt{
    R_{1,1} \ar[d] & \ar[l] K_{1,1} \dlcorner  \ar[d] \ar[r] & L_{1,1} \ar@{}[dr]|(.8){\text{\large $\ulcorner$}\qquad\quad} \ar[dr]^{f_1} && \ar[dl]_{f_2} \ar@{}[dl]|(.8){\qquad\quad\text{\large $\urcorner$}} L_{1,2} & \ar[l] K_{1,2} \ar[d] \drcorner\ar[r] & R_{1,2} \ar[d] \\
    G_{1,1}  & \ar[l] C_{1,1} \ar[rr] & & G_0  & & \ar[ll] C_{1,2}  \ar[r] & G_{1,2} \\
    &&& \ar@/^/[ull] I \ar[u] \ar@/_/[urr] & & &
    }$$

By epi-mono factorization of $[f_1,f_2]\colon L_{1,1}+L_{1,2} \to G_0$ we have
  $$ \vcenter{
    \xymatrix@R=15pt@C=5pt{
    L_{1,1} \ar[rd] \ar@(d,ul)[rdd]_{f_1} & & L_{1,2} \ar[ld] \ar@(d,ur)[ldd]^{f_2} \\
    & G_0' \ar@{_{(}->}[d] \\
    & G_0
    }
}$$
%\fgnote{sign mono arrows}

We apply Construction~\ref{constr:clipping} twice

$$ \scalebox{.8}{    \xymatrix@R=10pt@C=10pt{
  &  R_{1,1} \ar[dd]|\hole \ar[dl] & &  \ar[ll] K_{1,1} \ar[dl]  \ar[dd]|\hole \ar[rr] & &  L_{1,1} \ar[drr] \ar@/_1pc/[ddrr]|(.36)\hole && && \ar@/^1pc/[ddll]|(.36)\hole  L_{1,2} \ar[dll] & &  \ar[ll] K_{1,2}  \ar[dr] \ar[rr] \ar[dd]|\hole && R_{1,2} \ar[dr] \ar[dd]|\hole \\
  H_{1,1}' \ar[dr] && C_{1,1}' \ar[dr] \ar[ll]  \ar[rrrrr] & & & & & G_0' \ar[d] & & &&& C_{1,2}' \ar[dl]  \ar[lllll] \ar[rr] && H_{1,2}'   \ar[dl]\\
  &  H_{1,1}  & & \ar[ll] C_{1,1} \ar[rrrr] && & & G_0 && & & \ar[llll] C_{1,2}  \ar[rr] & & H_{1,2} \\
  & &&& &&& \ar@/^/[ullll] I \ar[u] \ar@/_/[urrrr] & & &
    }
}$$

Now $G_0'$ is a mda-hypergraph, since it is embedded into $G_0$ which is monogamous directed acyclic.
Therefore there exist some $J' \tr{f'} G_0'$ that is a mda-hypergraph with interface. We can apply twice Lemma \ref{lemma:keyconvex} to 
 $$ \scalebox{.8}{
    \xymatrix@R=10pt@C=10pt{
   K_{1,1}   \ar[rr]^{l_1} & &  L_{1,1} \ar[drr]^{f_1'}  && &&   L_{1,2} \ar[dll]_{f_2'} & &  \ar[ll]_{l_2} K_{1,2} \\
&  & & & G_0'   \\
 & &   & &  J' \ar[u]^{f'}
}}$$
since $l_i$ and $f_i'$ are mono for $i=1,2$. By uniqueness of pushout complement we have that there exists the span $C_{1,1}' \tl{} J' \to C_{1,2}'$ making the following diagram commute.
 $$ \scalebox{.8}{
    \xymatrix@R=10pt@C=10pt{
  &  R_{1,1}  \ar[dl] & &  \ar[ll] K_{1,1} \ar[dl]  \ar[rr] & &  L_{1,1} \ar[drr]  && &&   L_{1,2} \ar[dll] & &  \ar[ll] K_{1,2}  \ar[dr] \ar[rr]  && R_{1,2} \ar[dr] \\
  G_{1,1}'  && C_{1,1}'  \ar[ll]  \ar[rrrrr] & & & & & G_0'  & & &&& C_{1,2}'  \ar[lllll] \ar[rr] && G_{1,2}'   \\
  &   & &  && & & J' \ar[u]^{f'} \ar@/^5pt/[ulllll] \ar@/_5pt/[urrrrr] && & &    }
}$$
This is a pre-critical pair. By assumption it is joinable, i.e., we have derivations $$(G_{1,1}' \tl{} J') \DPOstep^* (W' \tl{\beta'} J' ) \DPOtlrewr (G_{1,2}' \tl{} J') \text{.}$$
Suppose that the leftmost derivation requires $n$ steps and the rightmost $m$. To keep the notation consistent with the embedding construction, we fix notation $G_{n,1}' \df W' {=:} \ G_{m,2}'$.

Now we would like to use now Construction~\ref{constr:embedding}, but first we need a general observation: in a mda-hypergraph with interface $H \tl{g} I$, $g$ is not mono iff $H$ contains some isolated node. Let us come back to our proof: since  $K_{1,i} \to L_{1,i}$ are mono for $i=1,2$, then $L_{1,i}$ do not contain any isolated node.  Also $G_0'$ do not contain an isolated node since $L_{1,1}+L_{1,2}\to G_0'$ is epi by construction.  Therefore $J_0' \tr{f'} G_0'$ is mono. Moreover, $m$ in the following diagram is mono by construction.
 $$ \scalebox{.8}{
    \xymatrix@R=10pt@C=10pt{
   J' \ar[r]^{f'}  & G_0' \ar[d]^m \\
I \ar[r]  & G_0   
}}$$
Therefore we can use Lemma \ref{lemma:keyconvex} to obtain 
\begin{equation*}
\begin{aligned}
\xymatrix{
& J' \ar[r]^{f'} \ar[d]_{\xi} \ar@{}[dr]|(.5){(\dagger)} & G_0' \ar[d]^m \\
I  \ar[r]^{\zeta}  \ar@/_10pt/[rr]_f 
& C  \ar[r] & G_0
}
\end{aligned}
\end{equation*}
and apply Construction~\ref{constr:embedding}, which yields
$$(G_0 \tl{} I) \DPOstep (G_{1,1} \tl{} I) \DPOstep^* (G_{n,1} \tl{\beta_1} I )$$
 extending $(G_0' \tl{} J') \DPOstep (G_{1,1}' \tl{} J') \DPOstep^* (G_{n,1}' \tl{\beta'} J' )$
   and
  $$(G_0 \tl{} I) \DPOstep (G_{1,2} \tl{} I) \DPOstep^* (G_{m,2} \tl{\beta_2} I)$$
   extending $(G_0' \tl{} J') \DPOstep (G_{1,1}' \tl{} J') \DPOstep^* (G_{m,2}' \tl{\beta'} J' )$.

 The next step is to prove that $(G_{n,1} \tl{\beta_1} I) \cong (G_{m,2} \tl{\beta_2} I) $. To see this, observe that both the following  squares are pushouts of 
 \[ C \tl{\xi} J' \tr{\beta'} W'=G_{n,1}'=G_{m,2}'.\]
 $$
 \xymatrix{
 J' \ar[d]_\xi \ar[r]^{\beta'} & G_{n,1}' \ar[d] \\
 C \ar[r]_{\beta_1'} & G_{n,1}
 }
 \qquad
 \xymatrix{
 J' \ar[d]_\xi \ar[r]^{\beta'} & G_{m,2}' \ar[d] \\
 C \ar[r]_{\beta_2'} & G_{m,2}
 }
$$
Indeed, the leftmost is a pushout by composition of squares $(\epsilon_n)$ and $(\delta_n)$ in the embedding construction and the rightmost by composition of $(\epsilon_m)$ and $(\delta_m)$. We conclude by observing that, by Construction~\ref{constr:embedding}, $\beta_i = \zeta ; \beta_i'$ for $i=1,2$. 
\end{proof}
