# Supplementary material for: String Diagram Rewrite Theory III: Confluence with and without Frobenius
Source: arXiv:2109.06049 source file (2022-04-18)
Supplement: Supplementary file 2 [file appendixConvexitySoundness.tex]

In order to prove Theorem \ref{thm:stronglyconnected}, we rely on a different rewriting mechanism -- called convex DPO rewriting -- that was introduced in \cite{BonchiGKSZ_lics16} and was shown to be sound and complete for every rewriting system (not necessarily left-connected) on $\syntax{\Sigma}$. 

\medskip

We need to recall some notions from \cite{BonchiGKSZ_lics16}.
A sub-hypergraph $H \subseteq G$ is \textit{convex} if, for any nodes $v, v'$ in $H$ and any directed path $e_1, \ldots, e_n$ from $v$ to $v'$ in $G$, every hyperedge in $e_i$ must also be in $H$. We call $m \colon L \to G$ in $\Hyp{\Sigma}$ a \textit{convex matching} if it is mono and its image is convex. For instance, the matchings in Example \ref{ex:unsoundcontext} are convex, while the matching in Example \ref{ex:unsound} is not: the path from $1$ to $3$ given by $\alpha_1, \alpha_3, \alpha_2$ is not in the image of $L$.

This formalises the notion of a subgraph `without holes', which corresponds exactly to the notion of a sub-expression in the syntax of a PROP. As shown by  Example \ref{ex:unsound}, non-convex matchings can lead to unsound rewriting in the absence of a chosen special Frobenius structure. However, restricting to convex matching is not enough to guarantee soundness of DPO with interfaces: we need to rule out also Example \ref{ex:unsoundcontext}. There are two possible ways: either restricting to systems with left-linear rules or restricting rewriting to \emph{boundary complements} \cite{BonchiGKSZ_lics16}. For the purposes of this paper, the first option is more convenient.

 \begin{defn}[Convex DPO rewriting step] \label{def:rigidDpoRewriting} Let $\mathcal{R}$ be a left-linear DPO rewriting system. A \emph{convex} DPO rewriting step  $(G\tl{} J )\rigidDPOstep{\mathcal{R}} (H\tl{} J ) $ is a DPO rewriting step with interface 
\begin{equation*}\label{eq:dpo3}
\raise25pt\hbox{$
\xymatrix@R=15pt@C=20pt{
L \ar[d]_{m}   &  K \ar[d]
 \ar@{}[dl]|(.8){\text{\large $\urcorner$}}
 \ar@{}[dr]|(.8){\text{\large $\ulcorner$}}
 \ar[l]_{} \ar[r]^{}  & R \ar[d] \\
 G &  C \ar[l] \ar[r]  & H \\
&  J \ar[u] \ar[ur]  \ar[ul]
}$}
\end{equation*}
where $(G \tl{}J)$ is a mda-hypergraph and $m \colon L \to G$ is a convex matching.
\end{defn}

The above definition coincides with the one in  \cite{BonchiGKSZ_lics16}, modulo the requirement that $C$ is a boundary complement. However, the restriction to left-linear rules entails that $C$ is uniquely determined by the matching $f$. Since, as shown in Lemma 3.11 in \cite{BonchiGKSZ_lics16}, a convex matching always induces a unique boundary complement, this should be exactly $C$. We can therefore rephrase Theorem 5.6 in \cite{BonchiGKSZ_lics16} as follows.

%
%\begin{theorem}\label{thm:stronglyconnected}
%Let $\mathcal{R}$ be a left-connected rewriting system on $\syntax{\Sigma}$.
%\begin{enumerate}
%\item If $d \rewr_\mathcal{R} e$, then $\rewiring{\SynToCsp{d}} \DPOstep_{\scriptscriptstyle{\rewiring{\SynToCsp{\mathcal{R}}}}}  \rewiring{\SynToCsp{e}}$.
%\item If $\rewiring{\SynToCsp{d}} \DPOstep_{\scriptscriptstyle{\rewiring{\SynToCsp{\mathcal{R}}}}}  (H\tl{}J)$, then $\exists e$ such that $\rewiring{\SynToCsp{e}}\cong (H\tl{}J)$ and $d \rewr_\mathcal{R} e$.
%\end{enumerate}
%\end{theorem}

\begin{theorem}\label{th:adequacyRigidSMT}Let $\mathcal{R}$ be a left-linear rewriting system on $\syntax{\Sigma}$.% containing a rule $\rrule{l}{r} \: (i,j)$.
\begin{enumerate}
\item If $d \rewr_\mathcal{R} e$, then $\rewiringsyn{d} \rigidDPOstep{\scriptscriptstyle{\rewiringsyn{\mathcal{R}}}}  \rewiringsyn{e}$.
\item If $\rewiringsyn{d} \rigidDPOstep{\scriptscriptstyle{\rewiringsyn{\mathcal{R}}}}  (H\tl{}J)$, then $\exists e$ such that $\rewiringsyn{e}\cong (H\tl{}J)$ and $d \rewr_\mathcal{R} e$.
\end{enumerate}
\end{theorem}
% OLD STATEMENT
%\begin{theorem}\label{th:adequacyRigidSMT}Let $\mathcal{R}$ be a left-linear rewriting system on $\syntax{\Sigma}$. Then, % containing a rule $\rrule{l}{r} \: (i,j)$.%the following are equivalent.
%\[
%d \rewr_{\mathcal{R}} e  \quad \text{ iff } \quad \rewiring{\SynToCsp{d}} \rigidDPOstep{\rewiring{\SynToCsp{\mathcal{R}}}}{\rewiring{\SynToCsp{e}}}\text{ .}
%\]
%\end{theorem}

The above part covers all the material that we need from  \cite{BonchiGKSZ_lics16}. We can now proceed with the proof of Theorem \ref{thm:stronglyconnected}. The key observation is that any matching of a strongly-connected mda-hypergraph into a larger mda-hypergraph must be convex.

\begin{lem}\label{lemma:connected->convex} Let $L \tl{} J \tr{} R$ be a left-linear strongly connected rule. Any matching $m\colon L \to G$ in a mda-hypergraph $G$ such that the square below is a pushout must be convex.
\[
\xymatrix{
L \ar[d]_{m} & \ar[l]_{i} J \ar[r] \ar[d] & R \\
G & \ar[l] C
}
\]
\end{lem}
\begin{proof} For $m$ being convex means that (i) $m$ is an embedding and (ii) the image of $m$ is a convex subgraph.

For (i), observe that the above square being a pushout implies that $m$ is injective on the edges of $L$: indeed, edges of $L$ could only be identified if they were in the image of $i \colon J \to L$, but $J$ is discrete. For nodes $n_1$ and $n_2$, we distinguish the following cases
where we write $n\in s(e)$ ($n\in t(e)$) iff there exists an $i$ such that $n=s_i(e)$ ($n= t_i(e)$).
\begin{itemize}
\item If $n_1 \in s(e_1)$ and $n_2 \in s(e_2)$, for some edges $e_1$ and $e_2$, then $m(e_1) \neq m(e_2)$ implies $m(n_1) \neq m(n_2)$, by monogamicity.
\item If $n_1 \in t(e_1)$ and $n_2 \in t(e_2)$, the same reasoning holds.
\item If $n_1 \in s(e_1)$ and $n_2 \in t(e_2)$, with $n_1$ input and $n_2$ output node, then identifying them would create a cycle in $G$.
\item If $n_1 \in s(e_1)$ and $n_2 \in t(e_2)$, with either $n_1$ not input or $n_2$ not output, then identifying them would violate monogamicity of $G$.
\item In the remaining case, one of the two nodes is neither in the source nor in the target of any edge, thus is both an input and an output. This cannot be the case, because $i$ must be a mono.
\end{itemize}
For (ii), take any two nodes $m(n_1)$ and $m(n_2)$ in the image of $m$ and consider a directed path $\pi$ from $m(n_1)$ to $m(n_2)$. Suppose for a contradiction that $\pi$ is not in the image of $m$. This mean that some segment $\tau$ of $\pi$ is not in the image of $m$, i.e.
$$m(n_1) \tr{\pi} m(n_2) = m(n_1) \tr{m(\sigma)} m(n_3) \tr{\tau} m(n_4)  \tr{m(\rho)} m(n_2).$$
Because both $G$ and $L$ are monogamous, then there is no outgoing edge in $L$ from $n_3$, and no ingoing edge in $L$ to $n_4$.  By monogamicity of $L$, this means that $n_3$ is an output node and $n_4$ is an input node of $L$. Therefore by strong connectedness there is a path $\pi'$ from $n_4$ to $n_3$ in $L$. But then the composite $m(\tau) ; \tau$ yields a cycle in $G$, contradiction. \end{proof}
%
%\begin{prop} \label{prop:connected->DPO=convex} Let $ G \tl{} J$ be a monogamous directed acyclic hypergraph with interface. For a left-linear strongly connected rule $L \tl{} K \tr{} R$, any DPO rewriting step
%\[
%\xymatrix@R=15pt@C=20pt{
%L \ar[d]   &  K \ar[d]
% \ar@{}[dl]|(.8){\text{\large $\urcorner$}}
% \ar@{}[dr]|(.8){\text{\large $\ulcorner$}}
% \ar[l] \ar[r]  & R \ar[d] \\
% G &  C \ar[l] \ar[r]  & H \\
%&  J \ar[u] \ar[ur]  \ar[ul]
%}
%\]
%is also a convex rewriting step.
%\end{prop}
%\fbnote{Aleks could you please check this carefully?}
%\fbnote{Why Sketch?}
%\fbnote{Maybe in the appendix we should insert the definitions of boundary complement and convex rewriting}
%\begin{proof}[proof sketch]
%There are two conditions to check. The first is that the matching $m$ is convex, which is guaranteed by Lemma~\ref{lemma:connected->convex}. The second is that $C$ is the boundary complement, see Definition 5.1 in \cite{LICS}. For that, the crucial observation is provided by Lemma 3.11 in \cite{LICS}: given a monogamous $G$ and a convex matching as above, it allows to decompose $G$ in terms of $L$ and its boundary complement $C'$. Because pushout complements are unique for left-injective rules, we can conclude that $C = C'$.
%\end{proof}

\begin{proof}[Proof of Theorem~\ref{thm:stronglyconnected}]
We have the following two steps.
\begin{enumerate}
\item If $d \rewr_\mathcal{R} e$ then, by Theorem \ref{th:adequacyRigidSMT},  $\rewiringsyn{d} \rigidDPOstep{\scriptscriptstyle{\rewiringsyn{\mathcal{R}}}}  \rewiringsyn{e}$ and then, by definition of  $\rigidDPOstep{\scriptscriptstyle{\rewiringsyn{\mathcal{R}}}}$, $\rewiringsyn{d} \DPOstep_{\scriptscriptstyle{\rewiringsyn{\mathcal{R}}}}  \rewiringsyn{e}$.
\item If $\rewiringsyn{d} \DPOstep_{\scriptscriptstyle{\rewiringsyn{\mathcal{R}}}}  (H\tl{}J)$ then, by  Lemma \ref{lemma:connected->convex}, $\rewiringsyn{d} \rigidDPOstep{\scriptscriptstyle{\rewiringsyn{\mathcal{R}}}}  (H\tl{}J)$ and, by Theorem \ref{th:adequacyRigidSMT}, $\exists e$ such that $\rewiringsyn{e}\cong (H\tl{}J)$ and $d \rewr_\mathcal{R} e$.
\end{enumerate}
%Observe that for a left-connected system we have:
%\[
%d \rewr_{\mathcal{R}} e  \quad \text{ iff } \quad \rewiring{\SynToCsp{d}} \rigidDPOstep{\rewiring{\SynToCsp{\mathcal{R}}}}{\rewiring{\SynToCsp{e}}} \quad \text{ iff }\quad \rewiring{\SynToCsp{d}} \DPOstep_{\rewiring{\SynToCsp{\mathcal{R}}}}{\rewiring{\SynToCsp{e}}} \text{ .}
%\]
%The first correspondence is given by Theorem \ref{th:adequacyRigidSMT} and the second by Lemma \ref{lemma:connected->convex}.
\end{proof}
