# Supplementary material for: String Diagram Rewrite Theory III: Confluence with and without Frobenius
Source: arXiv:2109.06049 source file (2022-04-18)
Supplement: Supplementary file 3 [file appendixExtraProofs.tex]

\begin{proof}[Proof of Lemma \ref{lem:decomp}] Pulling back~\eqref{eq:pushpull} along $m$,
we construct the following diagram, whose top face is precisely $(\dagger)$.
\[
\xymatrix@R=10pt@C=25pt{
& K \ar[ddl] \ar[d] \ar[rr] & & {C'} \ar[ddl]
\ar[d]^{id} \ar[rr]^{id} & & {C'} \ar[d] \ar[ddl] \\
& K \ar[ddl]|\hole \ar[rr]|(.75)\hole & & {C'} \ar[ddl]|\hole \ar[rr]|(.75)\hole & & C \ar[ddl] \\
L \ar[d] \ar[rr] & & {G'} \ar[rr]^{\id}
\ar[d]_{id} & & {G'} \ar[d]^(.2)m \\
L \ar[rr] & & {G'} \ar[rr]_m & & G
}
\]
Since pushouts are stable under pullback, 
$(\dagger)$ is a pushout as required. As both $(\ddagger)+(\dagger)$ and $(\dagger)$ are
pushouts, so is $(\ddagger)$ by the ordinary pushout pasting property.
\end{proof}

\begin{proof}[Proof of Lemma \ref{lemmacube}]
Let us show that the front right face is a pushout; the argument for the other front face is
symmetric. By assumption, the left rear face is a pullback,
thus $p$ is mono, since monos are stable under pullback in any category. We can conclude that this
face is thus a pushout along mono $p$, and hence Van Kampen.

Now, by assumption, the top and bottom faces are pullbacks, and the right rear face is a pullback.
It follows that the front face is also pullback: we can appeal to ordinary pullback pasting, since the commutativity of the cube
means that pasting the front face with the bottom face results in the same diagram as pasting the top and the rear right faces.
In adhesive categories pushouts along monos are stable under pullback, thus the front right face is a pushout.
\end{proof}
